# Supplementary material for: Containerized Distributed Value-Based Multi-Agent Reinforcement Learning
Source: arXiv:2110.08169 source file (2021-12-03)
Supplement: Supplementary file 1 [file AppendixD-ActionRepr.tex]

\section{Action Representation Learning}

As discussed in Sec. 5.1 of the main text, we use action representations to reduce the influence of utility difference function's estimation errors on graph structure learning. In this section, we describe the details of action representation learning (the related network structure is shown in Fig.~\ref{fig:action_repr_learner}). We
\begin{wrapfigure}[18]{r}{0.35\linewidth}
    \centering
    \includegraphics[width=\linewidth]{fig-demo/action_repr_learner.pdf}
    \caption{Framework for learning action representations, reproduced from~\cite{wang2021rode}.}
    \label{fig:action_repr_learner}
\end{wrapfigure}
use the technique proposed by~\citet{wang2021rode} and learn an action encoder $f_e(\cdot; \theta_e)$: $\mathbb{R}^{|A|}\rightarrow\mathbb{R}^d$, parameterized by $\theta_e$, to map one-hot actions to a $d$-dimensional representation space. With the encoder, each action $a$ has a latent representation $\vz_{a}$, \ie, $\vz_{a}=f_e(a; \theta_e)$. The representation $\vz_{a}$ is then used to predict the next observation $o_i'$ and the global reward $r$, given the current observation $o_i$ of an agent $i$, and the one-hot actions of other agents, $\va_{\shortn i}$. This model is a forward model, which is trained by minimizing the following loss:
\begin{equation}\label{equ:ar_learning}
\begin{aligned}
    \mathcal{L}_e(\theta_e, \xi_e) & = \mathbb{E}_{(\vo, \va, r, \vo')\sim \mathcal{D}}\big[\sum_i\|p_o(\vz_{a_i},o_i, \va_{\shortn i}) - o_i'\|^2_2 \\
    & + \lambda_e\sum_i\left(p_r(\vz_{a_i},o_i, \va_{\shortn i}) - r\right)^2\big],
\end{aligned}
\end{equation}
where $p_o$ and $p_r$ is the predictor for observations and rewards, respectively. We use $\xi_e$ to denote the parameters of $p_o$ and $p_r$. $\lambda_e$ is a scaling factor, $\mathcal{D}$ is a replay buffer, and the sum is carried out over all agents. 

In the beginning, we collect samples and train the predictive model shown in Fig.~\ref{fig:action_repr_learner} for 50$K$ timesteps. Then policy learning begins and action representations are kept fixed during training. Since tasks in the \bname~benchmark typically do not involve many actions, we do not use action representations when benchmarking our method. In contrast, StarCraft II micromanagement tasks usually have a large action space. For example, the map $\mathtt{MMM2}$ involves $16$ actions, and a conventional deep Q-network requires $256$ output heads for learning utility difference. Therefore, we equip our method with action representations to estimate the utility difference function when testing it on the SMAC benchmark.
