# Supplementary material for: Containerized Distributed Value-Based Multi-Agent Reinforcement Learning
Source: arXiv:2110.08169 source file (2021-12-03)
Supplement: Supplementary file 2 [file AppendixE-Hyper.tex]

\section{Architecture, Hyperparameters, and Infrastructure}
\subsection{\name}
In \name, each agent has a neural network to estimate its local utility. The local utility network consists of three layers---a fully-connected layer, a 64 bit GRU, and another fully-connected layer---and outputs an estimated utility for each action. The utility difference function is also a 3-layer network, with the first two layers shared with the local utility function to process local action-observation history. The input to the third layer (a fully-connected layer) is the concatenation of the output of two agents' GRU layer. The local utilities and pairwise utility differences are summed to estimate the global action value (Eq. 11 in the paper).

For all experiments, the optimization is conducted using RMSprop with a learning rate of $5\times10^{-4}$, $\alpha$ of 0.99, RMSProp epsilon of 0.00001, and with no momentum or weight decay. For exploration, we use $\epsilon$-greedy with $\epsilon$ annealed linearly from 1.0 to 0.05 over 50$K$ time steps and kept constant for the rest of the training. Batches of 32 episodes are sampled from the replay buffer. The default iteration number of the Max-Sum algorithm is set to 5. The communication threshold depends on the number of agents and the task, and we set it to $0.3$ on the map $\mathtt{5m\_vs\_6m}$ and $\mathtt{MMM2}$. We test the performance with different values ($1e\shortn 3$, $1e\shortn 4$, and $1e\shortn 5$) of the scaling weight of the sparseness loss $\mathcal{L}_{\text{sparse}}^{\delta_{\text{var}}}$ on $\mathtt{Pursuit}$, and set it to $1e\shortn 4$ for both the MACO and SMAC benchmark. The whole framework is trained end-to-end on fully unrolled episodes. All experiments on StarCraft II use the default reward and observation settings of the SMAC benchmark.

All the experiments are carried out on NVIDIA Tesla P100 GPU. We show the estimated running time of our method on different tasks in Table~\ref{tab:time-maco} and~\ref{tab:time-smac}. Typically, \name~can finish 1M training steps within 8 hours on \bname~tasks and in about 10 hours on SMAC tasks. In Table~\ref{tab:time-comparision}, we compare the computational complexity of action selection for CASEC and DCG, which is the bottleneck of both algorithms. CASEC is slightly faster than DCG by virtue of graph sparsity.

% \subsection{Baselines}
% We compare \name~with various baselines. For VDN \cite{sunehag2018value}, QMIX \cite{rashid2018qmix}, and DCG \cite{bohmer2020deep}, we use the codes provided by the authors where the hyperparameters have been fine-tuned on the SMAC benchmark.

\begin{table*}[h!]
    \caption{Approximate running time of \name~on tasks from the \bname~benchmark.}
    \centering
    \begin{tabular}{CRCRCRCRCRCR}
        \toprule
        \multicolumn{2}{c}{Aloha} &
        \multicolumn{2}{l}{Pursuit} &
        \multicolumn{2}{l}{Hallway} &
        \multicolumn{2}{l}{Sensor} &
        \multicolumn{2}{l}{Gather} &
        \multicolumn{2}{l}{Disperse} \\
        \cmidrule(lr){1-2}
        \cmidrule(lr){3-4}
        \cmidrule(lr){5-6}
        \cmidrule(lr){7-8}
        \cmidrule(lr){9-10}
        \cmidrule(lr){11-12}
        
        \multicolumn{2}{c}{13h (2M)} & \multicolumn{2}{c}{17h (2M)}  & \multicolumn{2}{c}{7h (1M)} & \multicolumn{2}{c}{4.5h (0.5M)} & \multicolumn{2}{l}{6.5h (1M)} & \multicolumn{2}{c}{8h (1M)}\\
        \toprule
    \end{tabular}
    \label{tab:time-maco}
    
    \caption{Approximate running time of \name~on tasks from the SMAC benchmark.}
    \centering
    \begin{tabular}{CRCRCRCRCR}
        \toprule
        \multicolumn{2}{l}{5m\_vs\_6m} &
        \multicolumn{2}{l}{MMM2}\\
        \cmidrule(lr){1-2}
        \cmidrule(lr){3-4}
        
        \multicolumn{2}{c}{18h (2M)} & \multicolumn{2}{c}{21h (2M)} \\
        \toprule
    \end{tabular}
    \label{tab:time-smac}
\end{table*}

\begin{table}[h!]
\centering
\caption{Average time (millisecond) for 1000 action selection phases of CASEC/DCG. CASEC uses a graph with sparseness 0.2 while DCG uses the full graph. To ensure a fair comparison, both Max-Sum/Max-Plus algorithms pass messages for 8 iterations. The batch size is set to 10.}
\vspace{0.5em}
\begin{tabular}{|c|c|c|c|}
  \hline
   &  5 actions & 10 actions & 15 actions \\ \hline
  5 agents & 2.90/3.11 & 3.15/3.39 & 3.42/3.67\\ \hline
  10 agents & 3.17/3.45 & 3.82/4.20 & 5.05/5.27 \\ \hline
  15 agents & 3.41/3.67 & 5.14/5.4  & 7.75/8.02 \\ \hline
\end{tabular}
\label{tab:time-comparision}
\end{table}
% \begin{table*}[t]
%     \caption{Approximate running time of \name~on tasks from the SMAC benchmark.}
%     \centering
%     \begin{tabular}{CRCRCRCRCRCR}
%         \toprule
%         \multicolumn{2}{c}{5m\_vs\_6m} &
%         \multicolumn{2}{l}{1c3s5z} &
%         \multicolumn{2}{l}{MMM2} &
%         \multicolumn{2}{l}{3s\_vs\_5z} &
%         \multicolumn{2}{l}{2c\_vs\_64zg} &
%         \multicolumn{2}{l}{2s\_vs\_1sc} \\
%         \cmidrule(lr){1-2}
%         \cmidrule(lr){3-4}
%         \cmidrule(lr){5-6}
%         \cmidrule(lr){7-8}
%         \cmidrule(lr){9-10}
%         \cmidrule(lr){11-12}
        
%         \multicolumn{2}{c}{24h (2M)} & \multicolumn{2}{c}{24h (2M)}  & \multicolumn{2}{c}{27h (2M)} & \multicolumn{2}{c}{24h (2M)} & \multicolumn{2}{l}{33h (2M)} & \multicolumn{2}{c}{24h (2M)}\\
%         \toprule
%     \end{tabular}
%     \label{tab:time-smac}
% \end{table*}
