# Supplementary material for: Containerized Distributed Value-Based Multi-Agent Reinforcement Learning
Source: arXiv:2110.08169 source file (2021-12-03)
Supplement: Supplementary file 3 [file AppendixC-SC2.tex]

% \begin{figure*}[ht]
%     \centering
%     \includegraphics[width=\linewidth]{fig-lc/smac_more.pdf}
%     \vspace{-2em}
%     \caption{Performance comparison against baselines and ablations on more SMAC tasks.}
%     \label{fig:smac_more-lc}
% \end{figure*}

\section{The SMAC benchmark}
On the SMAC benchmark, we compare our method against fully decomposed value function learning methods (VDN~\cite{sunehag2018value} \& QMIX~\cite{rashid2018qmix}) and a deep coordination graph learning method (DCG~\cite{bohmer2020deep}). Experiments are carried out on a hard map $\mathtt{5m\_vs\_6m}$ and a super hard map $\mathtt{MMM2}$. For the baselines, we use the code provided by the authors and their default hyper-parameters settings that have been fine-tuned on the SMAC benchmark. We also notice that both our method and all the considered baselines are implemented based on the open-sourced codebase PyMARL\footnote{https://github.com/oxwhirl/pymarl}, which further guarantees the fairness of the comparisons.
