# Supplementary material for: Containerized Distributed Value-Based Multi-Agent Reinforcement Learning
Source: arXiv:2110.08169 source file (2021-12-03)
Supplement: Supplementary file 4 [file AppendixF-Limitation.tex]

\section{Limitation}

An important advantage of learning sparse coordination graphs is reduced communication costs. In this paper, for each task, we set a fixed communication threshold then train and test our method. If we use a rather small threshold, fewer edges would be selected. In the early stage of training, when the utility difference function is not accurate, fewer edges may lead to worse action selections, rendering training unstable. To solve this problem, in our experiments, we select larger thresholds than necessary, which cannot fully reflect the power of context-aware sparse graphs. In future work, we plan to adaptively anneal the communication threshold during learning, automatically and accurately find the minimum threshold that can guarantee the learning performance.

Another limitation of our method is that the learned sparse graphs are not always cycle-free. Since the Max-Sum algorithm guarantees optimality only on acyclic graphs, our method may select sub-optimal actions. We plan to study how to solve this problem in future work.
